# Supplementary material for: Locating large flexible ligands on proteins
Source: arXiv:1707.02614 ancillary file (2017-07-11)
Supplement: Supplementary file 1 [file suppinf.pdf]

SUPPORTING INFORMATION

# Locating large flexible ligands on proteins

Jean-Noël Grad,[†] Alba Gigante,[‡] Christoph Wilms,[†] Jan Nikolaj Dybowski,[†] Ludwig Ohl,[†] Christian Ottmann,[¶] Carsten Schmuck,[‡] and Daniel Hoffmann[*,†]

*Bioinformatics and Computational Biophysics, Faculty of Biology, University of Duisburg-Essen, Universitätstraße 7, 45141 Essen, Germany, Institute of Organic Chemistry, University of Duisburg-Essen, Universitätstraße 7, 45141 Essen, Germany, and Laboratory of Chemical Biology, Department of Biomedical Engineering and Institute for Complex Molecular Systems, Eindhoven University of Technology, Den Dolech 2, 5612 AZ Eindhoven, The Netherlands*

E-mail: daniel.hoffmann@uni-due.de

Phone: +49 (0)201 183 4391. Fax: +49 (0)201 183 3437

[*] To whom correspondence should be addressed
[†] Bioinformatics and Computational Biophysics, Essen
[‡] Institute of Organic Chemistry, Essen
[¶] Biomedical Engineering, Eindhoven

## Input structures

Table S1: Geometries of the glycosaminoglycans used as input for EGs, following the crystallographic definition of the glycosidic angles $\Phi(i)$ ($O_{5(i)}$–$C_{1(i)}$–$O_{X(i-1)}$–$C_{X(i-1)}$) and $\Psi(i+i)$ ($C_{1(i+1)}$–$O_{1(i+1)}$–$C_{X(i)}$–$C_{X-1(i)}$) for aldopyranoses.[1] The two heparin structures were determined from a 2 µs MD simulation trajectory partitioned in two clusters. The other angles were based on the GlcNS-IdoA linkage in PDB entry 5t03.[2] The glycosidic bonds in heparan sulfate are known to be highly flexible,[3] so we checked the EG of the heparosan against the EG of an alternative conformer with different angles still within the experimental error, and found no significant difference. All sugar rings have the conformation $^4C_1$.

| Disaccharide unit | Linkage | $\Phi$ (°) | $\Psi$ (°) |
|---|---|---|---|
| Heparin (cluster 1) | GlcNS(6S)-IdoA(2S) | 63.7 | 95.0 |
| Heparin (cluster 2) | GlcNS(6S)-IdoA(2S) | 96.0 | 148.5 |
| Desulfated heparin | GlcNS-IdoA | 70.0 | 103.0 |
| Heparan sulfate | GlcNS-GlcA | 70.0 | 103.0 |
| Heparosan | GlcNAc-GlcA | 70.0 | 103.0 |
| Heparosan (alt.) | GlcNAc-GlcA | 100.0 | 79.0 |

heparin: 2-deoxy-4-*O*-methyl-2-(sulfoamino)-6-*O*-sulfonato-$\alpha$-D-glucopyranosyl-(1→4)-1-*O*-methyl-2-*O*-sulfonato-$\alpha$-L-idopyranuronate
desulfated heparin: 2-deoxy-4-*O*-methyl-2-(sulfoamino)-$\alpha$-D-glucopyranosyl-(1→4)-1-*O*-methyl-$\alpha$-L-idopyranuronate
heparan sulfate: 2-deoxy-4-*O*-methyl-2-(sulfoamino)-$\alpha$-D-glucopyranosyl-(1→4)-1-*O*-methyl-$\alpha$-D-glucopyranuronate
heparosan: 2-(acetamido)-2-deoxy-4-*O*-methyl-$\alpha$-D-glucopyranosyl-(1→4)-1-*O*-methyl-$\alpha$-D-glucopyranuronate

Table S2: PDB identifiers of crystal structures used as templates for refinement in Modeller and RMSD value between the templates and models.

| Protein | Template | RMSD (Å) |
|---|---|---|
| Sonic Hedgehog | 4c4n[4] | 0.30 |
| 14-3-3$\zeta$ | 4ihl[5] | 0.44 |
| $C_5$-epimerase | 4pw2[6] | 0.34 |
| Trp repressor | 1tro[7] | 0.36 |

Figure S1: Initial placement of QQJ-096 in the MD simulations with 14-3-3/c-Raf. Based on the EGs obtained in Figure 5, the search space was reduced to the 14-3-3 pore where the two c-Raf peptides are located. Two conformations of QQJ-096 extracted from a 50 ns simulation in water were introduced in the 14-3-3/c-Raf simulation box and rotated to yield 6 different starting conditions. In a first series of 6 simulations, the minimal distance between QQJ-096 and the c-Raf peptides was above 10 Å (A), however in 3 runs the ligand did not reach the receptor within 50 ns (C, upper panel). In a second series of 6 simulations, the ligand was brought closer to the pore, with a minimal distance of 4–6 Å (B), resulting in immediate binding (C, lower panel). The plateau at the beginning of the simulations (C) corresponds to the NVT equilibration where the coordinates of heavy atoms are restrained.

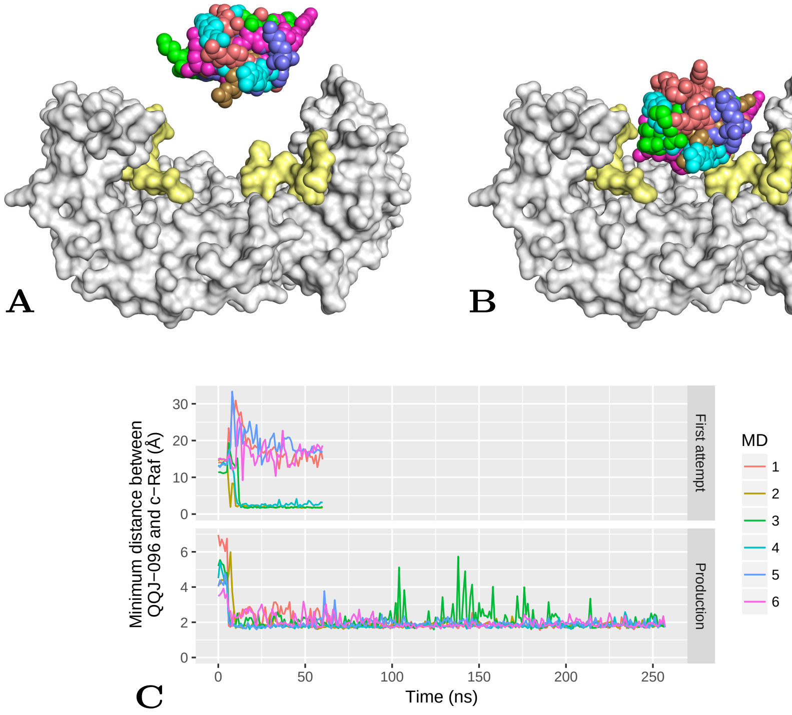

## Effect of different choices of parameters

Figure S2: Effect of the number of rotations $|\mathbf{\Omega}|$ on the quality of EGs of $C_5$-epimerase with a $CH_3O$-GlcNAc-GlcA-GlcNS-$OCH_3$ trisaccharide as molecular probe at a resolution of 0.8 Å. We measure the energy difference between grid points of an EG calculated with $|\mathbf{\Omega}|$ rotations and a reference EG with $|\mathbf{\Omega}| = 800$, while limiting ourselves to grid points where the molecular probe made contact with the protein surface, i.e. where $n$ angular states where allowed with $0 < n < |\mathbf{\Omega}|$. The average difference for any grid point in this region is close to zero with a 95% confidence interval decreasing as $|\mathbf{\Omega}|$ increases ($\pm 0.16\ k_{\mathrm{B}}T$ for $|\mathbf{\Omega}| = 75$, $\pm 0.10\ k_{\mathrm{B}}T$ for $|\mathbf{\Omega}| = 250$). The computation time increases linearly with $|\mathbf{\Omega}|$.

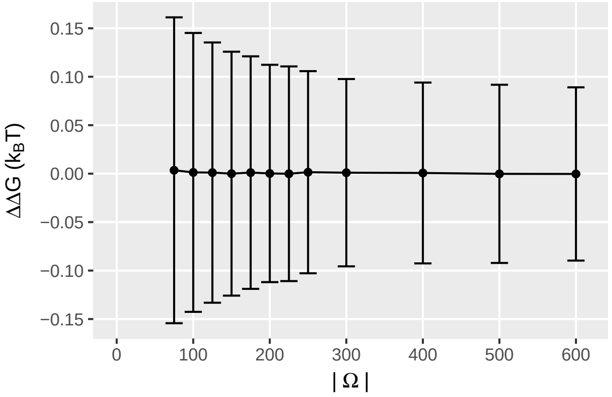


Figure S3: Effect of decreasing the grid size: EGs of $C_5$-epimerase scanned with the GlcNS-GlcA ligand at (A) 0.80 Å with penalty $\delta = -15$, (B) 0.40 Å with penalty $\delta = -3$, (C) 0.40 Å with penalty $\delta = -15$, all isosurfaces drawn at $\pm 1\ k_{\mathrm{B}}T$ (translucent blue/red) and $\pm 2\ k_{\mathrm{B}}T$ (solid blue/red) with black lines to represent the EG boundaries. The EG with $\delta = -3$ (A) shows slightly more detail but overall the same main structures as the EG with $\delta = -15$ (B). In contrast, details are lost if we increase resolution from 0.80 Å (A) to 0.40 Å (C) without adapting the penalty.

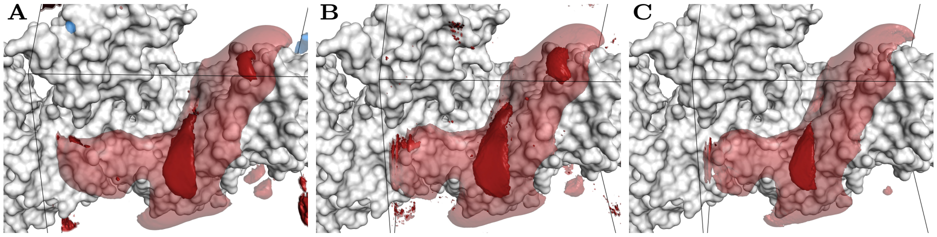


Figure S4: Effect of explicit water molecules: (A) Trp repressor (PDB entry 1tro [7]) with the crystallographic water molecules within 3 Å of the surface, (B) APBS grid without the water molecules, (C–D) epitopsy EGs using the crystallographic DNA fragment as molecular probe, with isosurfaces drawn at $-6\ k_{\mathrm{B}}T$ (translucent red) and $-8\ k_{\mathrm{B}}T$ (solid red), (C) without crystallographic waters and (D) with crystallographic waters.

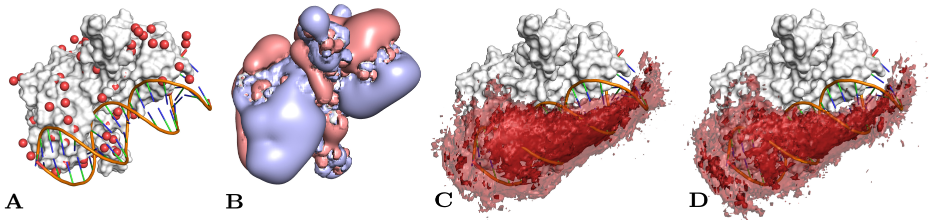

Figure S5: Effect of the ligand size: EGs of Sonic Hedgehog scanned with a heparin (A) dimer and (B) octamer, drawn at $-2\ k_{\mathrm{B}}T$ (translucent red) and $-4\ k_{\mathrm{B}}T$ (solid red), and ligand accessible surface (LAS) of the heparin (C) dimer and (D) octamer. The LAS in (D) is approximately 2 grid points larger than in (C), which corresponds to an 1.6 Å expansion. This offset can play an important role in protein surfaces with narrow clefts.

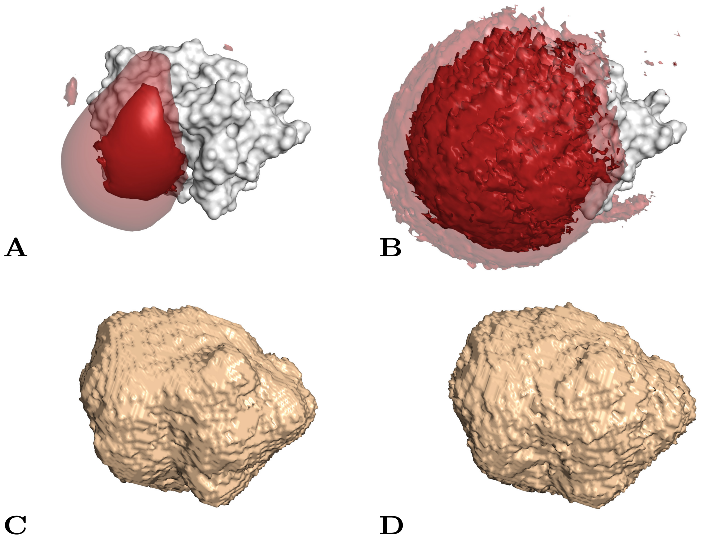


Figure S6: Effect of the ligand charge distribution: EGs of Sonic Hedgehog scanned with a heparin dimer with partial charges obtained (A) from GLYCAM and (B) from a manual assignment based on delocalized formal charges (charge -1/3 on sulfate oxygens and -1/2 on carboxylate oxygens, zero on everything else).

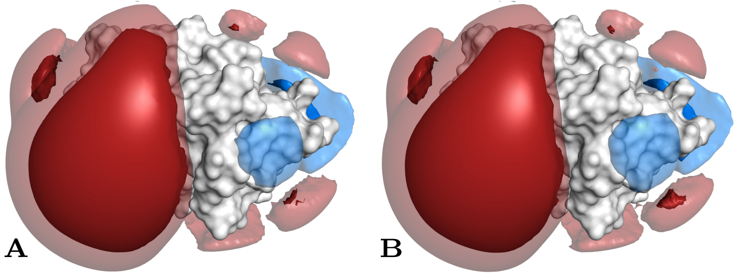

# MD trajectory clustering

Figure S7: Frequent binding sites on the surface of Sonic Hedgehog were extracted from the MD simulations using inter-residues, distance-based PCA.[8] The distances were computed as the minimum distance between basic amino acids in sonic hedgehog and negatively-charged groups ($R{-}SO_3^-$, $R{-}CO_2^-$) in heparin MD. Silhouette-validated PAM clustering of the binding sites was conducted on the first 6 principal components of the PCA matrix and yielded 4 clusters. (A) The 7 heparin trajectories projected into PCA space as dots colored by cluster. (B) Binding/unbinding events (spikes at 10–15 Å) are necessary for heparin to sample other binding sites. The still frames with no cluster information correspond to the 20 ns NVT equilibration with position restraints. (C) The 4 clusters are depicted as green spheres with radii logarithmically proportionnal to the cluster population, superimposed to the EG isosurfaces (Figure 2B, $\pm 1\ k_\mathrm{B}T$).

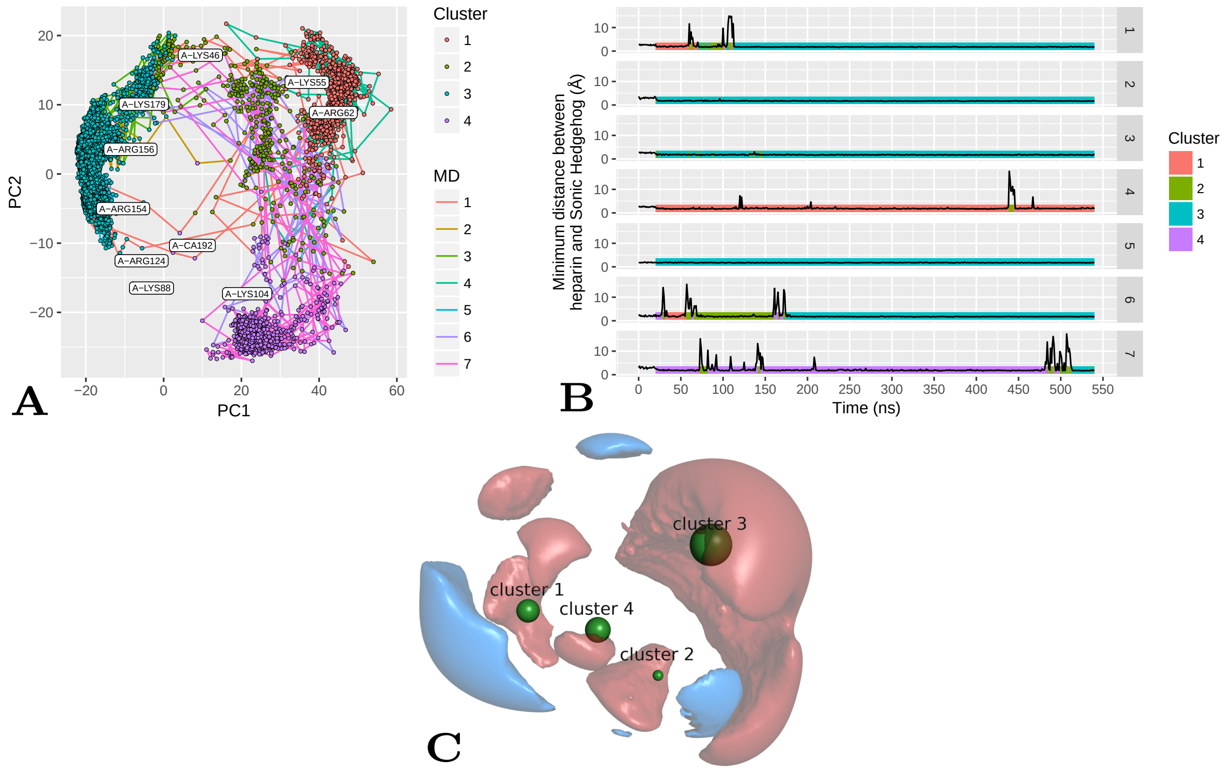

## ESP/EG correlation histograms

Figure S8: Correlation between the MD probability density and the ESP grid and EG of Sonic Hedgehog with a heparin dimer as molecular probe at a resolution of 0.8 Å. Attractive regions have positive potential in ESP and negative EG value. Binning the average MD occupancy versus the electrostatic potential resp. the energy in 2D histograms shows a higher correlation between EG and MD. In both histograms, the vertical line centered at zero corresponds to grid points far away from the protein, when the heparin was not making contact with the protein and was randomly navigating in water. The horizontal baseline in ESP corresponds to zones of high potential values never sampled in MD due to the van der Waals exclusion zone. The ESP distribution is slightly skewed towards grid points of positive energies, but the correlation is barely measurable. The Epitopsy distribution has two visible plumes in regions of negative energies. The second plot shows the MD occupancy on the log scale.

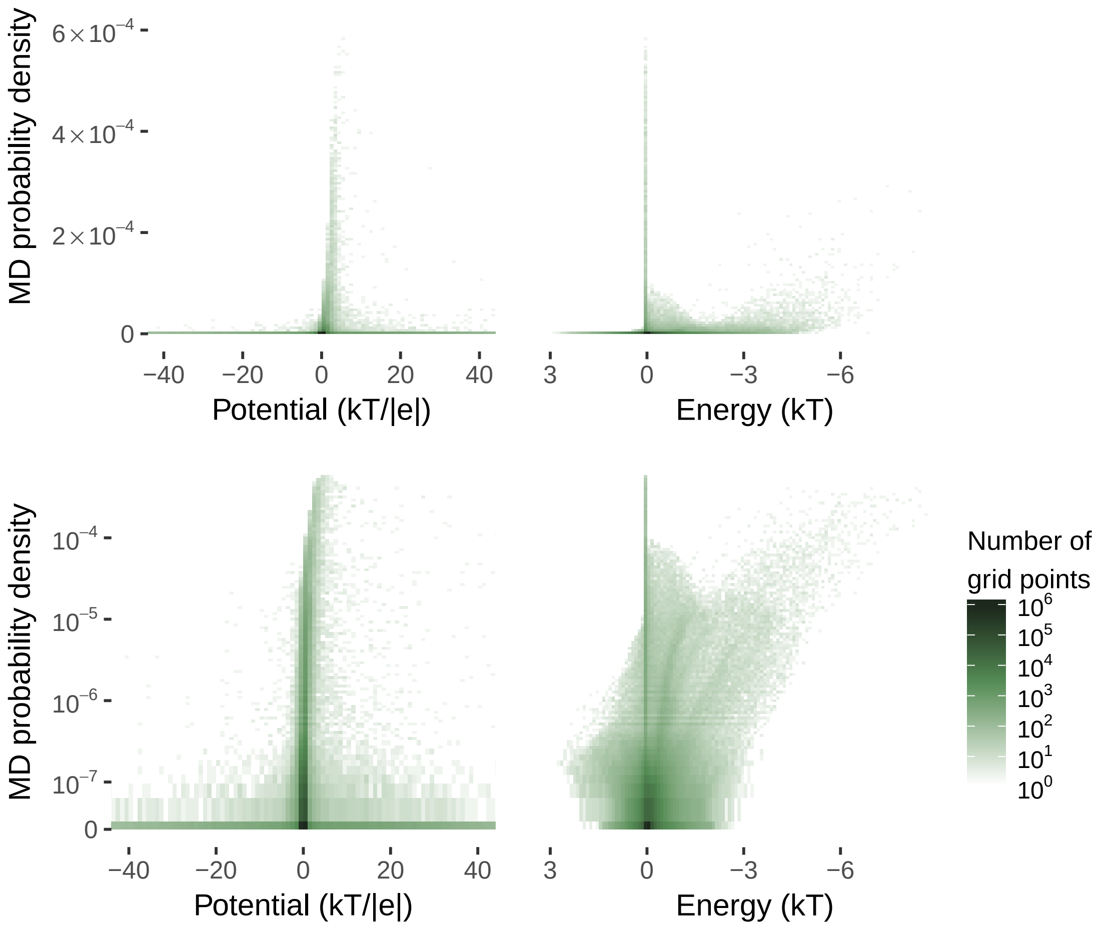

## References


(1) IUPAC, Symbols for Specifying the Conformation of Polysaccharide Chains. *European Journal of Biochemistry* **1983**, *131*, 5–7.

(2) Xu, Y.; Moon, A. F.; Xu, S.; Krahn, J. M.; Liu, J.; Pedersen, L. C. Structure Based Substrate Specificity Analysis of Heparan Sulfate 6-O-Sulfotransferases. *ACS chemical biology* **2017**, *12*, 73–82.

(3) Khan, S.; Fung, K. W.; Rodriguez, E.; Patel, R.; Gor, J.; Mulloy, B.; Perkins, S. J. The solution structure of heparan sulfate differs from that of heparin: implications for function. *The Journal of biological chemistry* **2013**, *288*, 27737–27751.

(4) Whalen, D. M.; Malinauskas, T.; Gilbert, R. J. C.; Siebold, C. Structural insights into proteoglycan-shaped Hedgehog signaling. *Proceedings of the National Academy of Sciences of the United States of America* **2013**, *110*, 16420–16425.

(5) Molzan, M.; Kasper, S.; Röglin, L.; Skwarczynska, M.; Sassa, T.; Inoue, T.; Breitenbuecher, F.; Ohkanda, J.; Kato, N.; Schuler, M.; Ottmann, C. Stabilization of physical RAF/14-3-3 interaction by cotylenin A as treatment strategy for RAS mutant cancers. *ACS chemical biology* **2013**, *8*, 1869–1875.

(6) Qin, Y.; Ke, J.; Gu, X.; Fang, J.; Wang, W.; Cong, Q.; Li, J.; Tan, J.; Brunzelle, J. S.; Zhang, C.; Jiang, Y.; Melcher, K.; Li, J.-p.; Xu, H. E.; Ding, K. Structural and functional study of D-glucuronyl C5-epimerase. *The Journal of biological chemistry* **2015**, *290*, 4620–4630.

(7) Otwinowski, Z.; Schevitz, R. W.; Zhang, R. G.; Lawson, C. L.; Joachimiak, A.; Marmorstein, R. Q.; Luisi, B. F.; Sigler, P. B. Crystal structure of trp repressor/operator complex at atomic resolution. *Nature* **1988**, *335*, 321–329.

(8) Ernst, M.; Sittel, F.; Stock, G. Contact- and distance-based principal component analysis of protein dynamics. *The Journal of chemical physics* **2015**, *143*, 244114.
